# Supplementary material for: Circum- and Inconic Invariants of 3-Periodics in the Elliptic Billiard
Source: arXiv:2004.02680 source file (2020-04-14)
Supplement: Supplementary file 1 [file 102_app_orbit_vertices.tex]

Let the boundary of the Billiard satisfy Equation~\eqref{eqn:billiard-f}. Assume, without loss of generality, that $a{\geq}b$.

Given a starting vertex $P_1$ and an exit angle $\alpha$ (as above), the orbit $P_1P_2P_3$ will be such that \cite{ronaldo19}:

vertex $P_2$ will be given by $(p_{2x},p_{2y})/q_2$, with

\begin{align*}
%\label{eqn:p2}
p_{2x}=&-{b}^{4} \left(  \left(   a^2+{b}^{2}\right)\cos^{2}\alpha   -{a}^{2}  \right) x_1^{3}-2\,{a}^{4}{b}^{2} \cos \alpha  \,\sin  \alpha  \,  x_1^{2}{y_1}\\
&+{a}^{4} \left(  ({a
}^{2}-3\, {b}^{2}) \cos^{2} \alpha  +{b}^{2}
 \right) {x_1}\,y_1^{2}-2{a}^{6} \,\cos  \alpha  \sin   \alpha  \, y_1^{3} ,
\\
p_{2y}=& 2{b}^{6} \,\cos \alpha\sin \alpha\,   x_1^{3}+{b}^{4}\left(  ({b
 }^{2}-3\, {a}^{2}) \cos^{2} \alpha  +{a}^{2}
  \right) x_1^{2}{y_1}\\
&+  2\,{a}^{2} {b}^{4}\cos \alpha \sin
  \alpha \; {x_1} y_1^{2} -{
a}^{4}  \left(  \left(   a^2+{b}^{2}\right)\cos^{2}  \alpha  -{b}^{2}  \right)  y_1^{3}
\\
q_2=&{b}^{4} \left( a^2-c^2\cos^2\alpha   \right)
x_1^{2}+{a}^{4} \left(  {b}^{2}+c^2\cos^2 \alpha  
 \right) y_1^{2}\\
 & - 2\, {a}^{2}{b}^{2}{c^2}\cos \alpha\sin \alpha \; {x_1}\,{
y_1}.
\end{align*}

and vertex $P_3$ will be given by $(p_{3x},p_{3y})/q_3$, with:

\begin{align*}
p_{3x}=& {b}^{4} \left( {a}^{2}- \left( {b}^{2}+{a}^{2} \right) \right)
 \cos^{2}  \alpha   x_1^{3} +2\,{a}^{4}{b}^{2} \cos  \alpha \sin \alpha\,   x_1^{2}{ y_1}\\
 &+{a}^{4} \left( 
  \cos^{2}  \alpha  \left( {a}^{2}-3\,{b}^{2}
 \right) +{b}^{2} \right) { x_1}\, y_1^{2} +2\, {a}^{6} 
 \cos \alpha\,\sin \alpha\, y_1^{3}
\\
p_{3y}=& -2\, {b}^{6} \cos \alpha\sin \alpha\, x_1^{3}+{b}^{4} \left( {a}^{2}+ \left( {b}^{2}-3\,{a}^{2} \right)    \cos^2\alpha \right) {{ x_1}}^{2}{ y_1}
\\
& -2\,{a}^{2}  {b}^{4}\cos
 \alpha  \sin \alpha\,  x_1 y_1^{2}+
 {a}^{4} \left( {b}^{2}- \left( {b}^{2}+{a}^{2} \right)   \cos^{2}  \alpha  \right)\,  y_1^{3},
\\
q_3=& {b}^{4} \left( {a}^{2}-{c^2}\cos^{2}\alpha   \right) x_1^{2}+{a}^{4} \left( {b}^{2}+c^2\cos^{2}\alpha  \right)  y_1^{2}\\
&+2\,{a}^{2}{b}^{
2} c^2 \cos\alpha \sin\alpha\, { x_1}\,{ y_1}.
\end{align*}

The sides of the triangular orbit have lengths 
$s_1=\mid P_3-P_2\mid$, $s_2=\mid P_3-P_1\mid$ and
$s_3=\mid P_2-P_1\mid$.
